# Supplementary material for: Adversarial Search and Tracking with Multiagent Reinforcement Learning in Sparsely Observable Environment
Source: arXiv:2306.11301 source file (2023-10-21)
Supplement: Supplementary file 1 [file appendix.tex]

\appendices 
\section{Filter Choice Validation}\label{sec:append}
\toedit{We propose that using a high-performance filter capable of accurately modeling the opponent's behavior will aid in faster convergence of agent policies trained with MARL in large domains. Therefore, we will first validate our PMC model by evaluating its accuracy and comparing with other baselines before applying it to MARL.}

\begin{figure}[t]
\label{fig:randomBlue}
	\centering
	\includegraphics[scale=0.3]{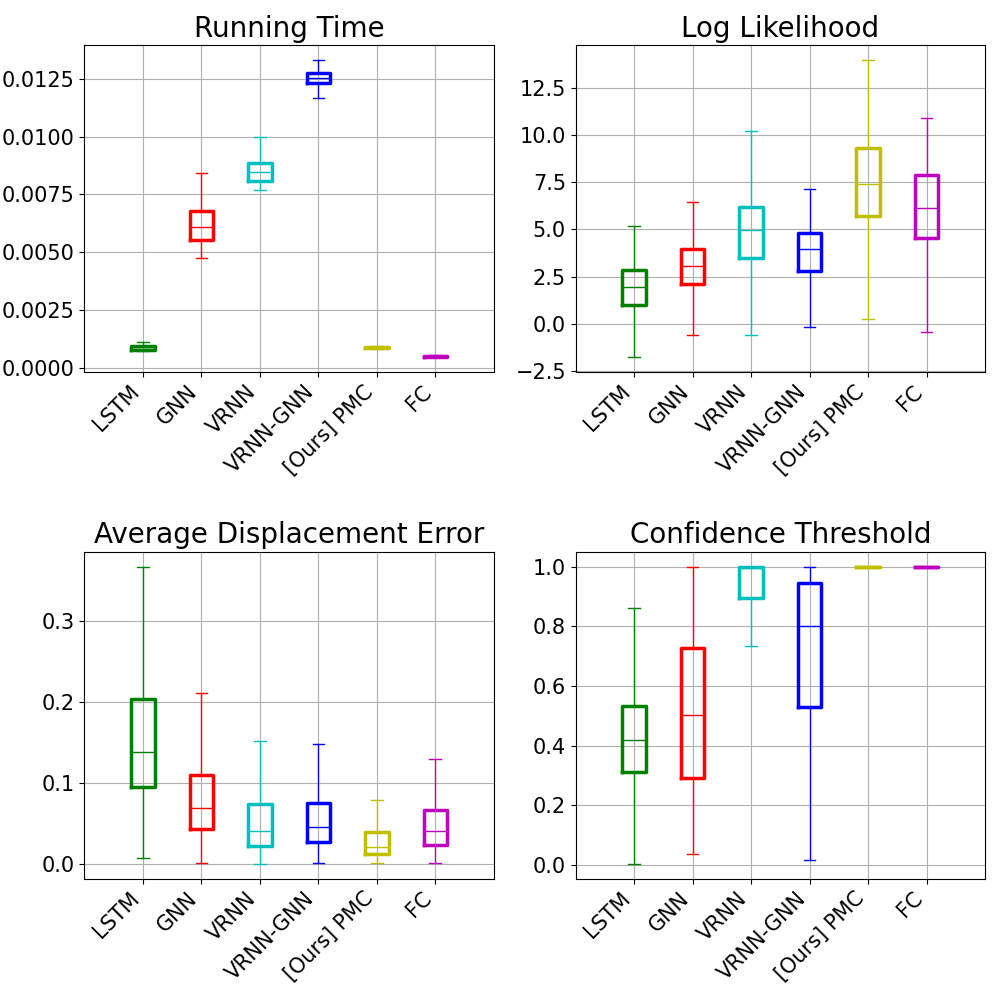}
 \vspace*{-0.5em}
	\caption{Multiple Filter Evaluations with Random Searching Policy \toedit{(Higher is better except for Average Displacement Error and Running Time)}}
    \label{fig:random_filter}
    \vspace*{-0.15in}
\end{figure}

\begin{figure}[t]
\label{fig:heuBlue}
	\centering
	\includegraphics[scale=0.3]{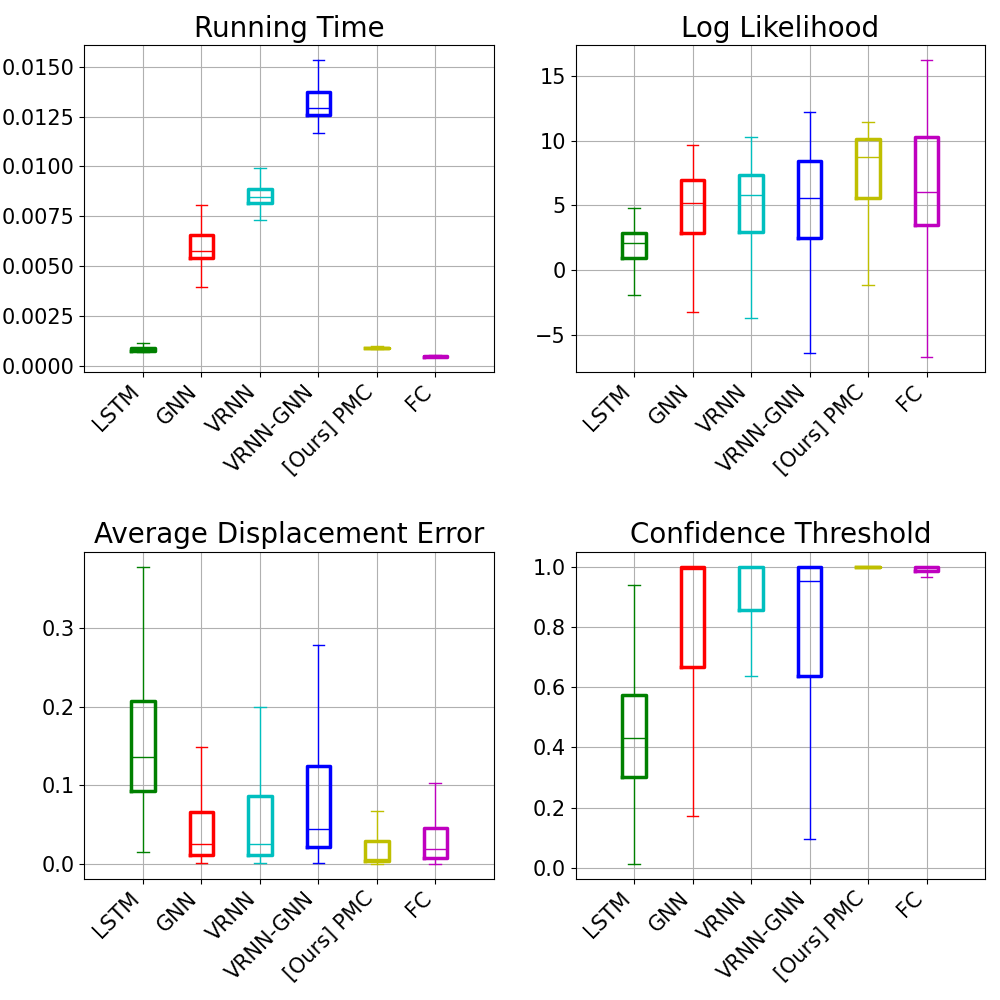}
 \vspace*{-0.5em}
	\caption{Multiple Filter Evaluations with Heuristic Searching Policy \toedit{(Higher is better except for Average Displacement Error and Running Time)}}
    \label{fig:heuristic_filter}
      \vspace*{-0.15in}
\end{figure}

\toedit{We evaluate our PMC filter with four RNN-based filter configurations (LSTM, VRNN  GNN, VRNN-GNN) and one FC configuration with metrics running time (RT), Log-Likelihood (LL), Average Displacement Error (ADE), and Confidence Threshold (CTP). LL estimates the log-likelihood between the predicted gaussian distribution and the adversary location. ADE is the $l_2$ distance between the mean of the predicted distribution and the adversary location. CTP is the ratio of timesteps for which the model predicts the probability of adversary location is greater than $0.5$. All the filter configurations follow an encoder-decoder structure where the encoder is either an LSTM, a graph neural network (GNN), a variational RNN (VRNN), VRNN with graph (VRNN-GNN), or fully connected (FC) network and the decoder is a FC layer outputs the Gaussian parameters. The input for all RNN based filtering approaches includes the detection histories of all agents for the last 16 timesteps with the last two detection appended. Both PMC and FC models are using the same source of input (last two detections with velocities, current timesteps and starting locations) with relatively small networks. We trained on the dataset with 300 trajectories where the searching agents are using random policy (see Figure \ref{fig:random_filter}) and heuristic (see Figure \ref{fig:heuristic_filter}) respectively. Results on 200 evaluation trajectories clearly shows that PMC and FC models perform better than others so we try to use them as informing filters in our MARL framework.}
